# Supplementary material for: Locally finite two-loop amplitudes for electroweak production through gluon fusion
Source: arXiv:2403.13712 source file (2024-11-12)

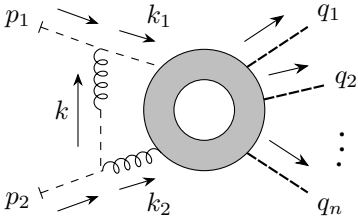

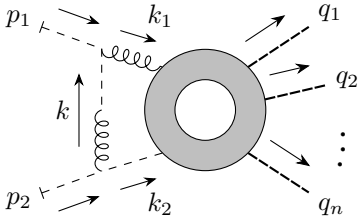

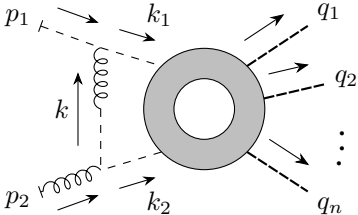

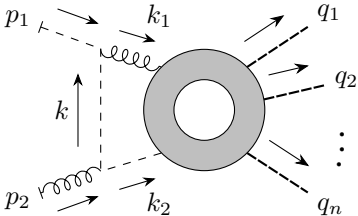

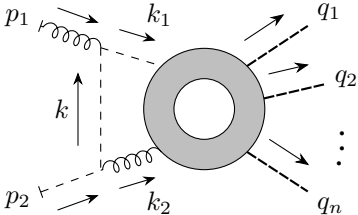

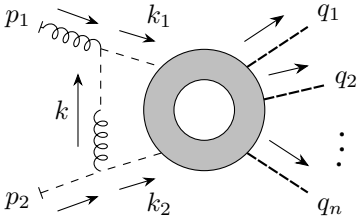

Supplement: Supplementary file 1 [file tikz_diag_appendix.pdf]
